# Supplementary material for: Reversible Markov chain estimation using convex-concave programming
Source: arXiv:1603.01640 source file (2016-03-04)
Supplement: Supplementary file 1 [file appendix.tex]

\appendix

\section{Gradients and Hessians \label{sec:grad_and_hess}}
